# Supplementary material for: Entropy-Stable Schemes in the Low-Mach-Number Regime: Flux-Preconditioning, Entropy Breakdowns, and Entropy Transfers
Source: arXiv:2110.11941 source file (2022-01-06)
Supplement: Supplementary file 1 [file Appendix_LSA.tex]

For a first-order explicit scheme, linear stability is achieved \cite{Birken} if the complex amplification matrix $H$ defined by:
\begin{equation*}
    H = I - \nu((\cos(\phi) - 1) D - i \sin(\phi) A), \ \nu = \frac{\Delta t}{\Delta x}, \ i^2 = -1,
\end{equation*}
has a spectral radius $\rho(H) \leq 1, \ \forall \phi$ ($D$ is the dissipation matrix, $A$ is the system Jacobian). For simplicity, we work with (\ref{LMES:eq:2b2}):
\begin{equation*}
    A = \begin{bmatrix} 
        u & a/M_r \\
        a/M_r & u
        \end{bmatrix} = R \Lambda R^{-1}, \ \Lambda = \begin{bmatrix} 
            u + a/M_r & 0 \\
            0 & u - a/M_r
        \end{bmatrix}, \ R = 
        \begin{bmatrix}
            1 & 1 \\
            1 & -1
        \end{bmatrix}.
\end{equation*}
The skewed dissipation operator we introduced in section \ref{LMES:dS_scheme}) writes:
\begin{equation*}
    D = R |\Lambda_P| R^{-1}, \ |\Lambda_P| =  \begin{bmatrix}
    f_1 (u+a/M_r) & 0 \\ 0 & f_2 (a/M_r - u)
    \end{bmatrix}
    + \begin{bmatrix}
    0 & \delta \\ - \delta & 0
    \end{bmatrix}
    .
\end{equation*}
Taking $f_1 = |u| / (u + a/M_r)$, $|u| / (a/M_r - u)$, and $\delta = a/M_r$ gives:
\begin{equation*}
    D = \begin{bmatrix}
    |u| & -a/M_r \\
    a/M_r & |u|
    \end{bmatrix},
\end{equation*}
which scales like $A$. To inspect the spectral radius of $H$ we consider the matrix $\widetilde{H}$ defined by the similarity transformation:
\begin{equation*}
    \widetilde{H} = R^{-1} H R =  I - \nu((c - 1) \Lambda_P - i s \Lambda) = \begin{bmatrix}
    1 - \nu(c-1) |u| + i \nu s (u+a/M_r) & - \nu (c-1)a/M_r \\
    \nu (c - 1) a/M_r & 1 - \nu(c-1) |u| + i \nu s (u - a/M_r)
    \end{bmatrix},
\end{equation*}
where $c = \cos(\phi)$ and $s = \sin(\phi)$. $\widetilde{H}$ has two complex eigenvalues $\lambda_1 $ and $\lambda_2$ given by:
\begin{equation*}
    \lambda_1 = 1 + \nu |u| (c-1) + i  \nu  ((a/M_r) \sqrt{2(1-c)} + s u) , \ \lambda_2 = 1 + \nu |u| (c-1) - i  \nu  ((a/M_r) \sqrt{2 (1-c)} - s u).
\end{equation*}
If $c = 1$, then $s = 0$ and $\Lambda_{1,2} = 1$. For $c \neq 1$, we have:
\begin{equation*}
    \lambda_{1,2}^2 = 1 - 2 (1-c) \nu  \big( |u| - \nu (u^2+(a/M_r)^2 \pm s (a/M_r) u \sqrt{2/(1-c)}) \big). 
\end{equation*}
$\lambda_{1,2}^2 \leq 1$ imposes:
\begin{equation*}
2 (1-c) \nu  \big( |u| - \nu (u^2+(a/M_r)^2 \pm s (a/M_r) u \sqrt{2/(1-c)}) \big) \geq 0 \ \Leftrightarrow \nu \leq \frac{ M_r^2 |u|}{M_r^2 u^2+a^2 \pm s M_r a u \sqrt{2/(1-c)}} = \mathcal{O}(M_r^2).
\end{equation*}
This shows that the linearized scheme with $D$ has a more restrictive CFL condition ($\nu = \mathcal{O}(M_r^2)$) than with the classic upwind operator ($\nu = \mathcal{O}(M_r)$). If the skew term is removed, a similar CFL condition is obtained:
\begin{equation*}
    \nu < \frac{M_r^2 |u|}{ M_r^2 u^2 + a^2 (c+1)/2 \pm (c+1) M_r a u} = \mathcal{O}(M_r^2).
\end{equation*}
