# Supplementary material for: Entropy-Stable Schemes in the Low-Mach-Number Regime: Flux-Preconditioning, Entropy Breakdowns, and Entropy Transfers
Source: arXiv:2110.11941 source file (2022-01-06)
Supplement: Supplementary file 2 [file Appendix_Central.tex]

\indent As established analytically in \cite{ES_Tadmor_1987} and numerically in \cite{Miczek_T, Miczek}, the central flux alone is not a viable option in the low Mach regime because it is not stable even when combined with Backward Euler in time. An illustration is provided in figure \ref{fig:gresho_central}-(b), which shows losses in total entropy, and in figure \ref{fig:gresho_central}-(a), which shows that the central flux leads to total kinetic energy production (Gresho Vortex). With the EC flux, the total entropy increases and the total kinetic energy fluctuates but does not become bigger than what it was initially. 
\begin{figure}[!htbp]
    \centering
    \subfigure[Total kinetic energy $ k/k_0$]{\includegraphics[scale = 0.68]{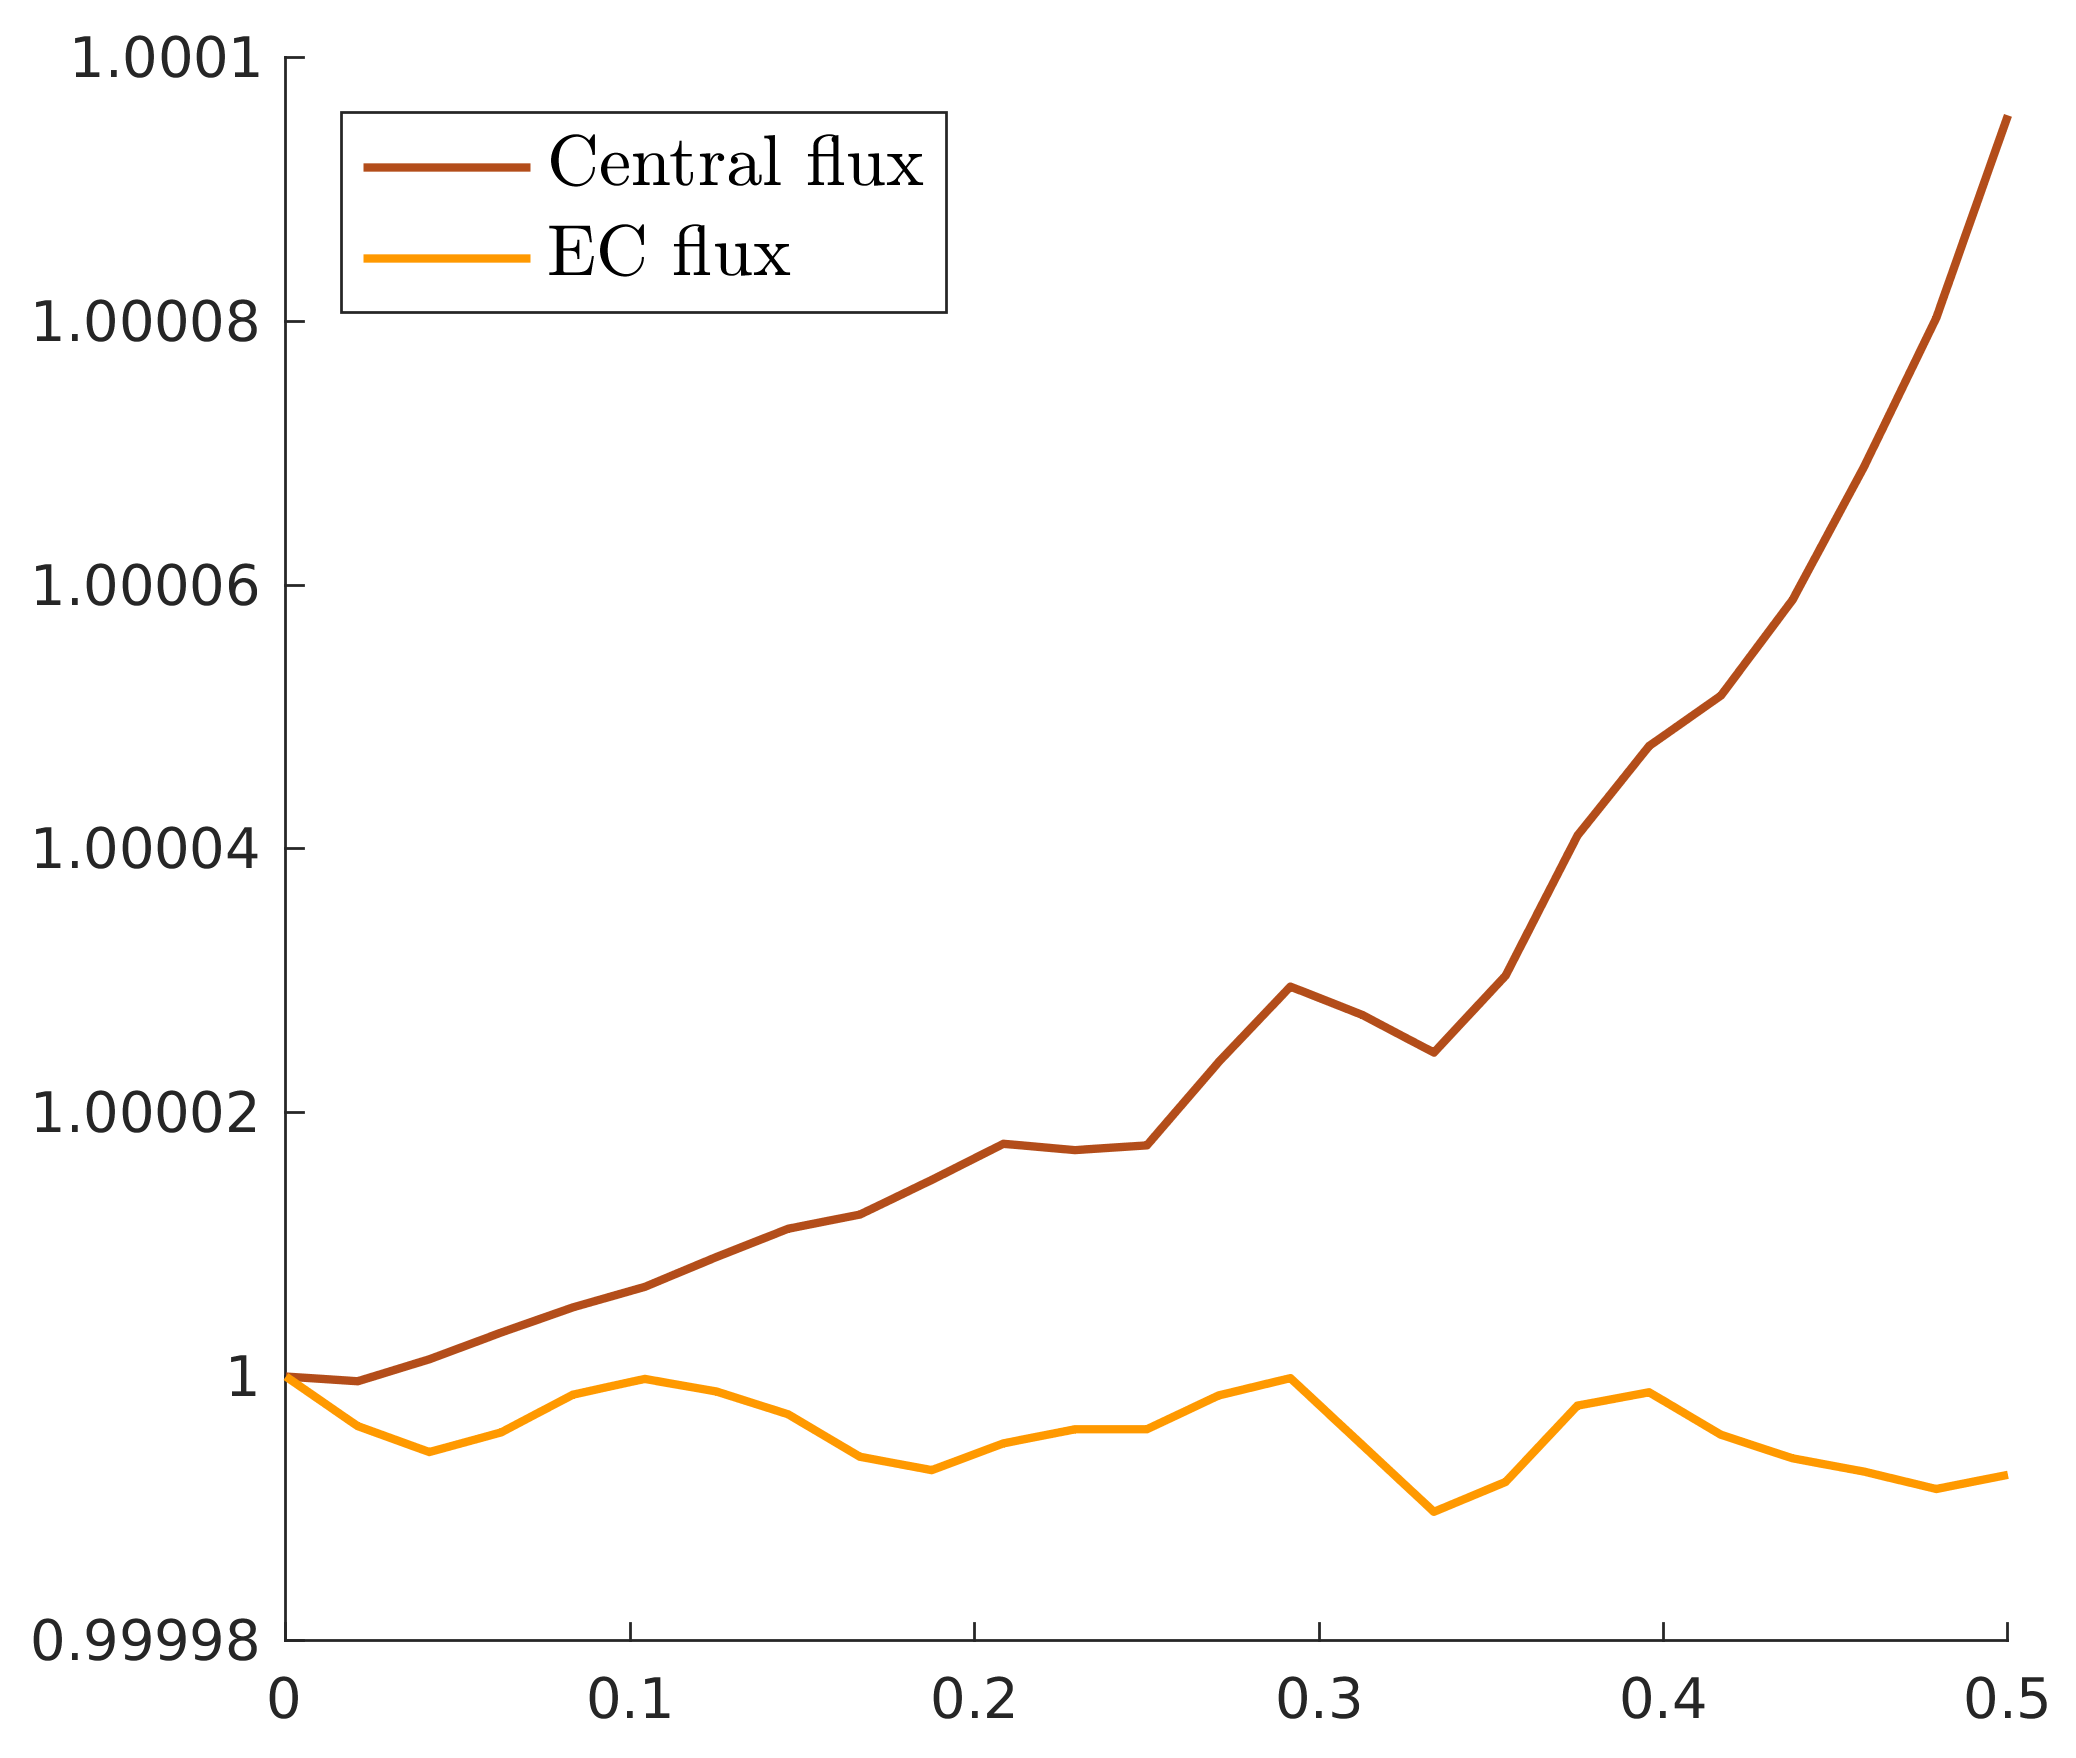}}
    \subfigure[Total Entropy $ (\rho s) - (\rho s)_0$]{\includegraphics[scale = 0.68]{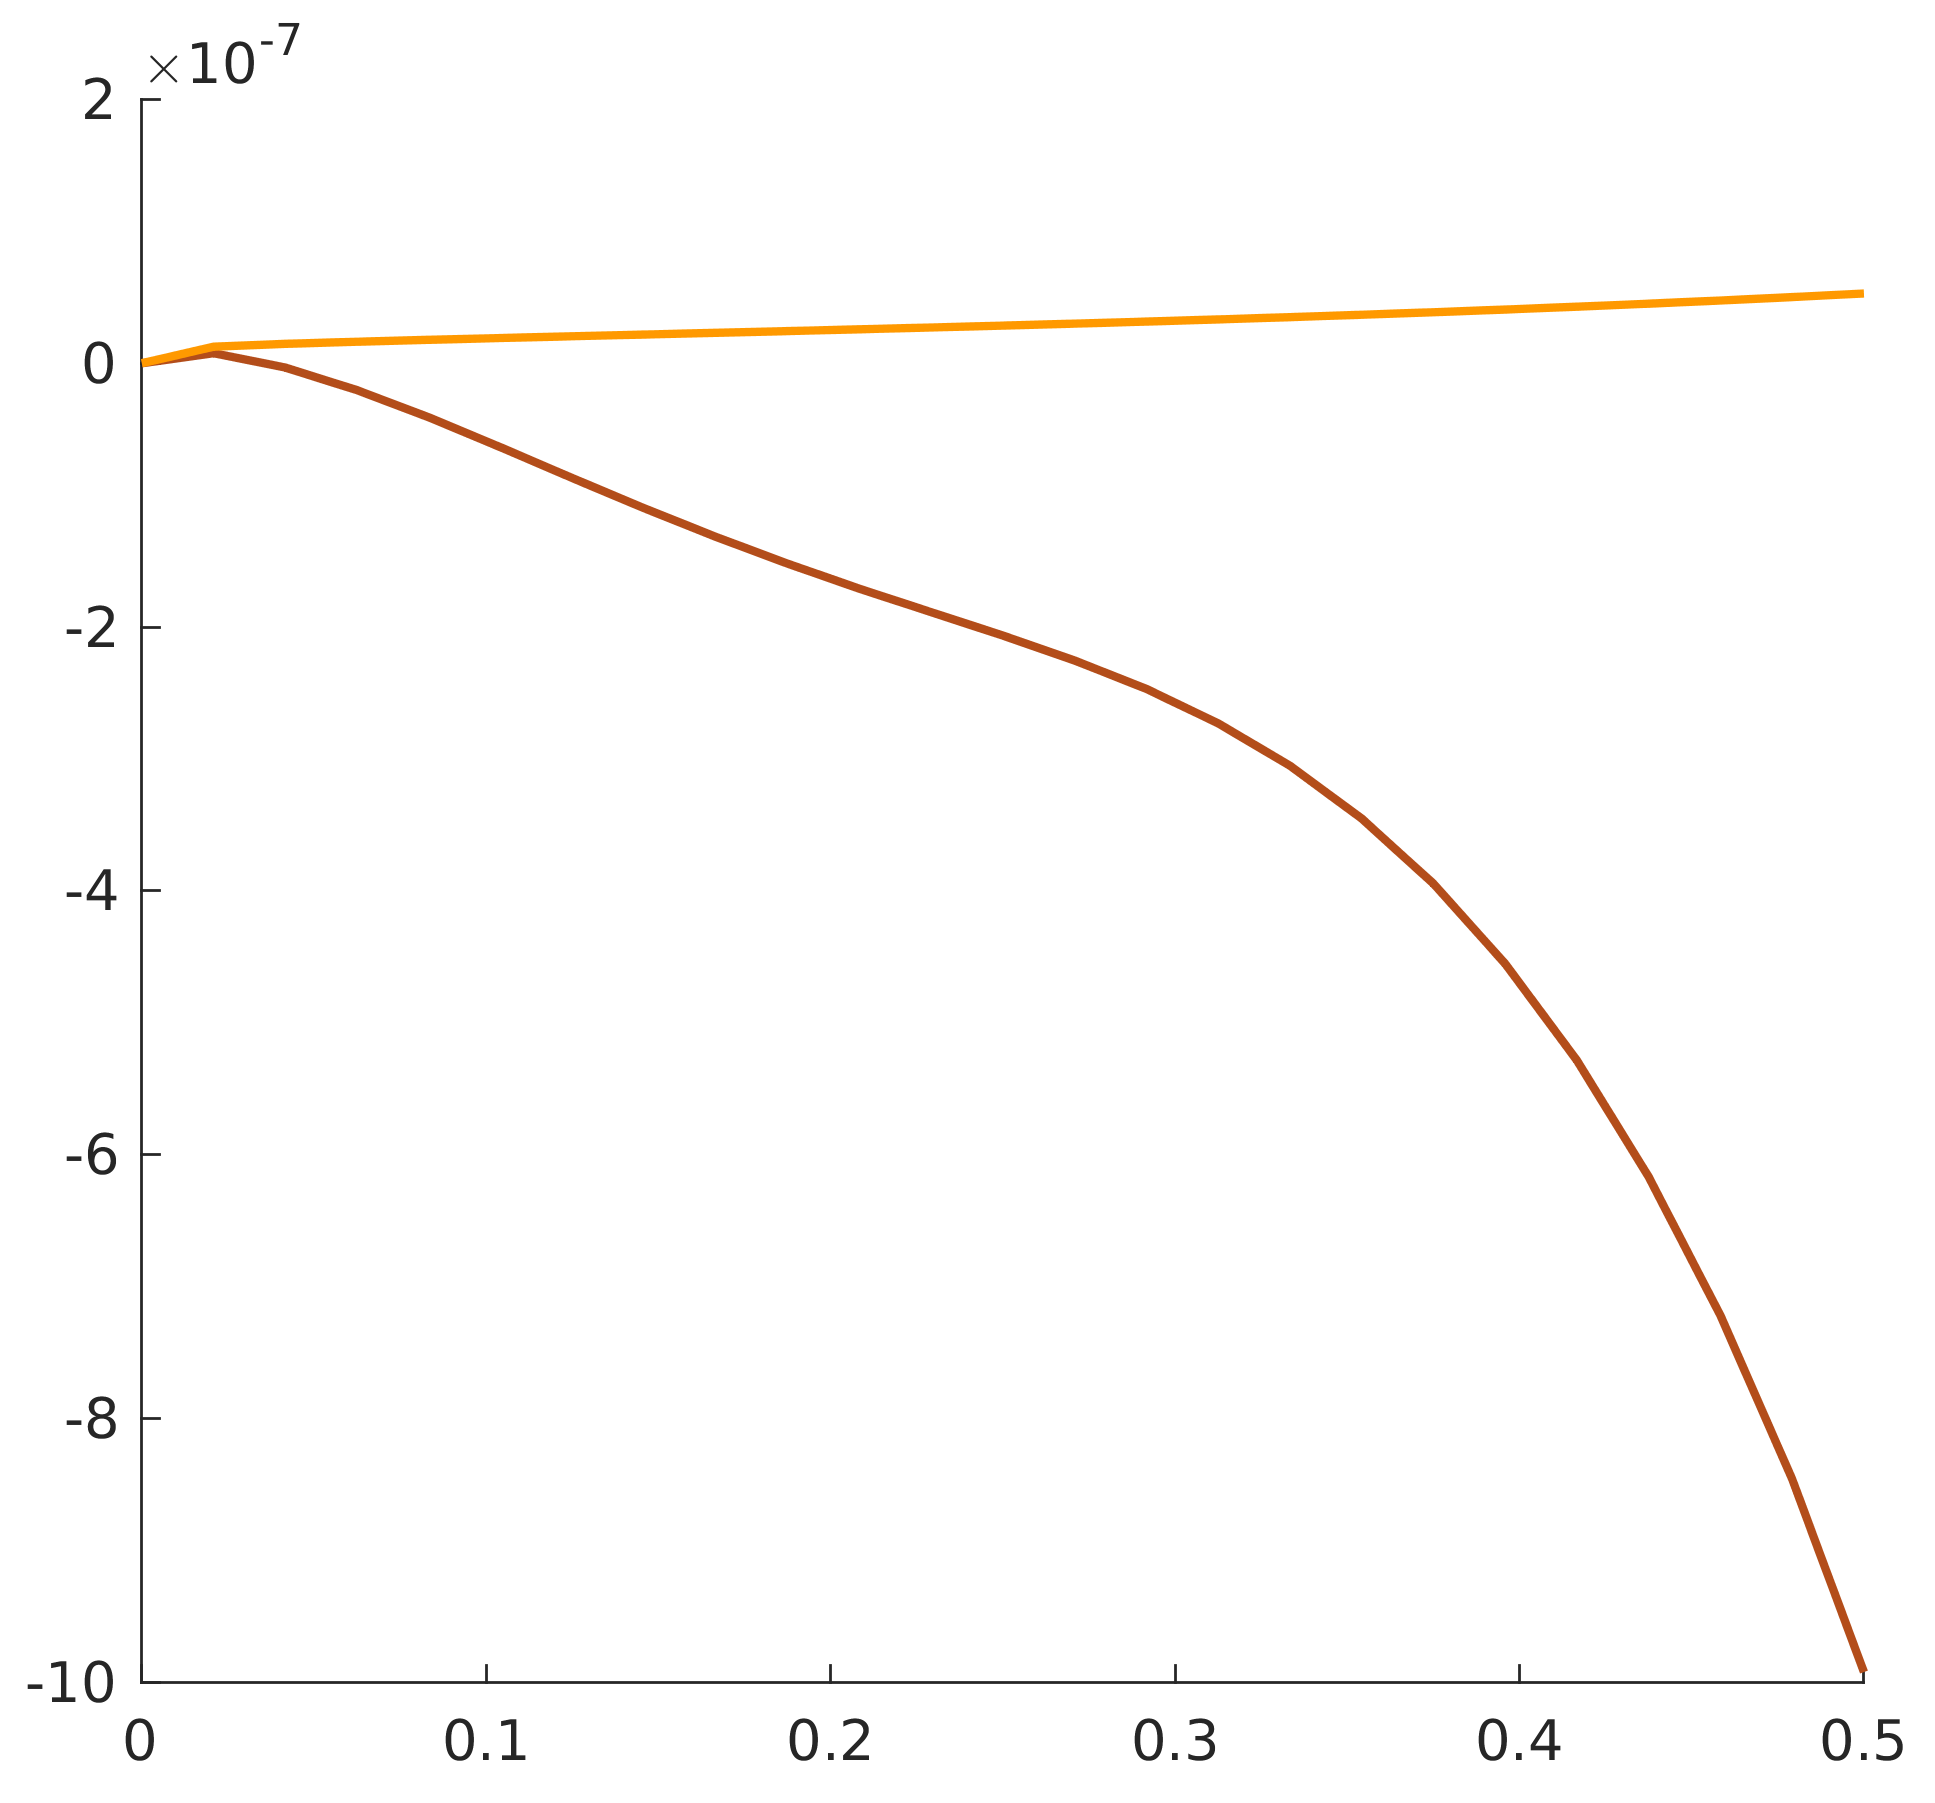}}
    \caption{Kinetic energy and entropy evolution with the central and EC fluxes in space and Backward Euler in time for half a rotation of the Gresho vortex at $M_r = 3 \times 10^{-1}$. $k_0$ and $(\rho s)_0$ are the kinetic energy and entropy at $t = 0$.}
    \label{fig:gresho_central}
\end{figure}
