# Supplementary material for: Entropy-Stable Schemes in the Low-Mach-Number Regime: Flux-Preconditioning, Entropy Breakdowns, and Entropy Transfers
Source: arXiv:2110.11941 source file (2022-01-06)
Supplement: Supplementary file 3 [file Appendix_ES.tex]

\indent The dimensional form of Chandrasekhar's EC flux and of the standard ES dissipation operator $R|\Lambda|R^{T}[\mathbf{v}]$ is obtained by setting $M_r = 1$ in (\ref{eq:EC_Chandra}), and (), respectively.   \\
\indent The dimensional form of the preconditioned ES dissipation operators are not as straightforward as blabla. can be evaluated in two equivalent ways.
